# Supplementary material for: Enhancing Model Robustness and Fairness with Causality: A Regularization Approach
Source: arXiv:2110.00911 source file (2021-10-03)
Supplement: Supplementary file 1 [file appendix.tex]

We provide supplemental information in this section.

\subsection{Results using weighted Glove embeddings \notezw{BERT}}
\begin{table*}[h]
    \centering \small
    \begin{tabular}{l l l| l l | l l} 
    \hline
      & & & \multicolumn{2}{c|}{{\bf IMDB}} & \multicolumn{2}{c}{{\bf Kindle}} \\
         \cline{4-7}
        
         {\bf causal} & {\bf spurious} & {\bf remain} & {\bf Test} & {\bf CTF}  & {\bf Test} & {\bf CTF} \\
         \hline
         1 & 1 & 1 & 0.824 $\pm$ 0.002 & 0.619 $\pm$ 0.006 & 0.822 $\pm$ 0.004 & 0.553 $\pm$ 0.027 \\
         \hline
         10 & 1 & 1 & 0.804 $\pm$ 0.009 & \colorbox{brown!30}{0.754 $\pm$ 0.002} & 0.761 $\pm$ 0.041 & 0.542 $\pm$ 0.046 \\
         1 & 0.1 & 1 & 0.824 $\pm$ 0.004 & 0.648 $\pm$ 0.004 & 0.794 $\pm$ 0.008 & \colorbox{brown!30}{0.583 $\pm$ 0.017} \\
         1 & 1 & 0.1 & 0.816 $\pm$ 0.004 & 0.603 $\pm$ 0.005 & 0.814 $\pm$ 0.004 & 0.539 $\pm$ 0.007 \\
         10 & 0.1 & 1 & 0.804 $\pm$ 0.009 & \colorbox{brown!30}{0.755 $\pm$ 0.003} & 0.793 $\pm$ 0.005 & \colorbox{brown!30}{0.580 $\pm$ 0.011} \\
         10 & 1 & 0.1 & 0.786 $\pm$ 0.011 & \colorbox{brown!30}{0.743 $\pm$ 0.005} & 0.790 $\pm$ 0.016 & 0.525 $\pm$ 0.024 \\
         \hline
    \end{tabular}
    \caption{Glove embedding + LR: Robustness evaluation (accuracy reported) for tuned classifier on test and Counterfactual (CTF) data for IMDB and Kindle dataset. Results in upper table are based on causal features identified from top coefficient terms and lower part uses causal features identified from the whole vocabulary.}
    \label{tab.CTF_robust}
\end{table*}
